# Supplementary material for: Semi-supervised multiple testing
Source: arXiv:2106.13501 source file (2021-11-24)
Supplement: Supplementary file 1 [file MR2021supp_arxiv2.pdf]

# Supplement to "Semi-supervised multiple testing"

**David Mary**

*Université Côte d'Azur, Observatoire de la Côte d'Azur, CNRS, Laboratoire Lagrange, Bd de l'Observatoire, CS 34229, 06304, Nice cedex 4, France*
*e-mail:* david.mary@oca.eu

**Etienne Roquain**

*Sorbonne Université (Université Pierre et Marie Curie), LPSM, 4, Place Jussieu, 75252 Paris cedex 05, France*
*e-mail:* etienne.roquain@upmc.fr

**Abstract:** This supplement contains additional materials for the main paper: proofs of the main results; auxiliary results and additional numerical experiments.

## Contents

S1 Proof of Theorem 3.1 . . . 1
S1.1 Reformulation of $\widehat{\mathrm{BH}}$ . . . 1
S1.2 Randomization lemma . . . 2
S1.3 Core argument for the proof . . . 2
S1.4 Super-martingale argument . . . 3
S1.5 Proof of Lemma S3 . . . 4
S2 Proofs for power results . . . 5
S2.1 Proof of Proposition 4.1 . . . 5
S2.2 Proof of Proposition 4.2 . . . 6
S2.3 Proof of Proposition 4.3 . . . 7
S2.4 Proof of Theorem 5.1 . . . 8
S3 Auxiliary results . . . 10
S4 Additional numerical experiments . . . 12
S4.1 Comparison to naive procedures . . . 12
S4.2 Results in a non Gaussian case . . . 12
S4.3 Results for small values of $n$ . . . 12
S4.4 Results for bbBH procedure . . . 12
References . . . 14

## S1. Proof of Theorem 3.1

We assume throughout the proof that $\mathcal{H}_0 = \{1, \dots, m_0\}$ without loss of generality.

### *S1.1. Reformulation of $\widehat{BH}$*

Let us reformulate $\widehat{\mathrm{BH}}$ according to Algorithm 1, which will be useful for the proof. For this, let us order the $Z_i$'s, that is, $Z_{\tau(1)} \geq \dots \geq Z_{\tau(n+m)}$ and consider $s_\ell = \mathbb{1}_{\{\tau(\ell) \leq n\}} \in \{0, 1\}$, $1 \leq \ell \leq n+m$, which is 1 if and only if $Z_{\tau(\ell)}$ comes from sample $Y = (Y_1, \dots, Y_n)$. Then, we easily see that $\widehat{\mathrm{BH}}_\alpha$ reject $H_i$ if $X_i \geq Z_{\tau(\hat{\ell})}$ where

$$\hat{\ell} = \max\left\{\ell \in \{1, \dots, n+m\} \,:\, \widehat{\mathrm{FDP}}_\ell \leq \alpha\right\}, \quad \widehat{\mathrm{FDP}}_\ell = \frac{m}{n+1} \frac{1 + \sum_{\ell'=1}^{\ell} s_{\ell'}}{1 \vee \sum_{\ell'=1}^{\ell}(1 - s_{\ell'})}, \tag{S1}$$



imsart-generic ver. 2014/10/16 file: MR2021supp_arxiv2.tex date: November 24, 2021

with no rejection if this set is empty.

### S1.2. Randomization lemma

First, let us provide two lemmas that will be useful for the proof. Consider the null sample $W = (Y_1, \dots, Y_n, X_1, \dots, X_{m_0})$ of size $n+m_0$. Consider $\pi$ the permutation of $\{1, \dots, n+m_0\}$ that orders the $W_i$'s in decreasing order, that is, $W_{\pi(1)} \geq \dots \geq W_{\pi(n+m_0)}$ and let $s_{0,\ell} = \mathbb{1}_{\{\pi(\ell) \leq n\}} \in \{0, 1\}$ for any $\ell \in \{1, \dots, n+m_0\}$ which equals 1 if and only if $W_{\pi(\ell)}$ comes from the sample $Y$. Under (Exch), since the $W_i$'s are exchangeable and $F_0$ is continuous, there is almost surely no tie in the sample $W$ and $\pi$ is uniformly distributed among all permutations of $\{1, \dots, n+m_0\}$. Hence, the following lemma holds.

**Lemma S1.** *Under* (Exch)*, the set* $S_0 = \{\ell \in \{1, \dots, n+m_0\} : s_{0,\ell} = 1\}$ *is uniformly distributed among all subset of* $\{1, \dots, n+m_0\}$ *of cardinality* $n$ *and this, independently from the order statistics* $(W_{\pi(1)}, \dots, W_{\pi(n+m_0)})$*, and of* $(X_i, m_0+1 \leq i \leq m)$*.*

To study the new procedure, we should now make the link between $s_{0,\ell}$ and $s_\ell$. Denote

$$L = \{\ell \in \{1, \dots, n+m\} : \tau(\ell) \leq n+m_0\}. \tag{S2}$$

The integer $L$ corresponds to the ordered indices of the $Z_i$'s coming from the $Y_i$'s. Then we map $\{1, \dots, n+m_0\}$ to $L$ by using a bijection only depending on the order statistics $(W_{\pi(1)}, \dots, W_{\pi(n+m_0)})$ and $(X_i, m_0+1 \leq i \leq m)$, and thus a bijection independent of $S_0$. Hence, the above lemma entails the following result.

**Lemma S2.** *Under* (Exch)*, the set* $S = \{\ell \in L : s_\ell = 1\}$ *is uniformly distributed among all subsets of* $L$ *of cardinality* $n$ *and this, independently from the order statistics* $(W_{\pi(1)}, \dots, W_{\pi(n+m_0)})$ *and of* $(X_i, m_0+1 \leq i \leq m)$*.*

Also note that $s_\ell = 0$ when $\ell \notin L$, and we introduce the following notation:

$$V_\ell = \sum_{1 \leq \ell' \leq \ell, \ell' \in L} s_{\ell'} = \sum_{1 \leq \ell' \leq \ell} s_{\ell'}, \text{ for all } \ell \in \{1, \dots, n+m\}. \tag{S3}$$

### S1.3. Core argument for the proof

When $\widehat{\mathrm{BH}}_\alpha$ makes at least one rejection, $\hat{\ell} \in \{1, \dots, n+m\}$ exists. Let in addition $\hat{\ell} = 0$ when $\widehat{\mathrm{BH}}_\alpha$ makes no rejection. When $\hat{\ell} > 0$, we also denote $\hat{t} = Z_{\tau(\hat{\ell})}$. Now, by definition,

$$\begin{aligned} \mathrm{FDR}(P, \widehat{\mathrm{BH}}_\alpha) &= \mathbb{E}[\mathrm{FDP}(P, \widehat{\mathrm{BH}}_\alpha)] = \mathbb{E}[\mathrm{FDP}(P, \widehat{\mathrm{BH}}_\alpha) \mathbb{1}_{\{\hat{\ell} > 0\}}] \\ &= \mathbb{E}\left[ \frac{\sum_{i \in \mathcal{H}_0} \mathbb{1}_{\{X_i \geq \hat{t}\}}}{1 \vee \sum_{i=1}^m \mathbb{1}_{\{X_i \geq \hat{t}\}}} \mathbb{1}_{\{\hat{\ell} > 0\}} \right]. \end{aligned} \tag{S4}$$

Now, relying on (S1), we have almost surely

$$\begin{aligned} \frac{\sum_{i \in \mathcal{H}_0} \mathbb{1}_{\{X_i \geq \hat{t}\}}}{1 \vee \sum_{i=1}^m \mathbb{1}_{\{X_i \geq \hat{t}\}}} \mathbb{1}_{\{\hat{\ell} > 0\}} &= \frac{n+1}{m} \frac{\sum_{i \in \mathcal{H}_0} \mathbb{1}_{\{X_i \geq \hat{t}\}}}{\sum_{i=1}^n \mathbb{1}_{\{Y_i \geq \hat{t}\}} + 1} \frac{m}{n+1} \frac{\sum_{i=1}^n \mathbb{1}_{\{Y_i \geq \hat{t}\}} + 1}{1 \vee \sum_{i=1}^m \mathbb{1}_{\{X_i \geq \hat{t}\}}} \mathbb{1}_{\{\hat{\ell} > 0\}} \\ &= \frac{m_0}{m} \widehat{\mathrm{FDP}}_{\hat{\ell}} \times \frac{n+1}{m_0} \frac{\sum_{i \in \mathcal{H}_0} \mathbb{1}_{\{X_i \geq \hat{t}\}}}{\sum_{i=1}^n \mathbb{1}_{\{Y_i \geq \hat{t}\}} + 1} \mathbb{1}_{\{\hat{\ell} > 0\}}, \end{aligned} \tag{S5}$$

In the next section, we will prove the following equality:

$$\mathbb{E}\left[ \frac{n+1}{m_0} \frac{\sum_{i \in \mathcal{H}_0} \mathbb{1}_{\{X_i \geq \hat{t}\}}}{\sum_{i=1}^n \mathbb{1}_{\{Y_i \geq \hat{t}\}} + 1} \mathbb{1}_{\{\hat{\ell} > 0\}} \right] = 1. \tag{S6}$$

Let us check that this implies the statements of Theorem 3.1: first, since by definition $\widehat{\mathrm{FDP}}_{\hat\ell} \leq \alpha$ when $\hat\ell > 0$, relations (S4)-(S5)-(S6) implies $\mathrm{FDR}(P, \widehat{\mathrm{BH}}_\alpha) \leq \frac{m_0}{m}\alpha$. Second, if $\alpha(n+1)/m$ is an integer, we have $\widehat{\mathrm{FDP}}_{\hat\ell} = \alpha$ when $\hat\ell > 0$ by Lemma S4, hence relations (S4)-(S5)-(S6) implies $\mathrm{FDR}(P, \widehat{\mathrm{BH}}_\alpha) = \frac{m_0}{m}\alpha$. Finally, Lemma S5 gives $\widehat{\mathrm{FDP}}_{\hat\ell} \geq \frac{m}{n+1}\lfloor \alpha\frac{n+1}{m}\rfloor$ when $\hat\ell > 0$, which gives $\mathrm{FDR}(P, \widehat{\mathrm{BH}}_\alpha) \geq \frac{m_0}{m}\frac{m}{n+1}\lfloor \alpha\frac{n+1}{m}\rfloor$.

### *S1.4. Super-martingale argument*

Let $\xi = ((W_{\pi(1)}, \ldots, W_{\pi(n+m_0)}), (X_i, i > n+m_0))$ for short. The proof is based on a super-martingale argument. Recall the equivalent definition (S1), so that (S6) is proved if

$$\mathbb{E}\left[M_{\hat\ell}\mathbb{1}_{\{\hat\ell\geq 1\}} \mid \xi\right] = \frac{m_0}{n+1},\ \ M_\ell = \frac{\sum_{\ell\in L, 1\leq \ell'\leq \ell}(1-s_{\ell'})}{\sum_{\ell'\in L, 1\leq \ell'\leq \ell} s_{\ell'} + 1} = \frac{m_{0,\ell} - V_\ell}{V_\ell + 1}, 1 \leq \ell \leq m+n, \tag{S7}$$

where $V_\ell$ is given by (S3) and $m_{0,\ell}$ denotes the cardinal of $\{1 \leq \ell' \leq \ell : \ell' \in L\}$ for $1 \leq \ell \leq m+n$. By Lemma S2, the randomness in the above expectation is only carried by the binary variable $(s_\ell, \ell \in L)$ for which $S = \{\ell \in L : s_\ell = 1\}$ is uniformly distributed among all subset of $L$ of cardinality $n$, conditionally on $\xi$ ($L$ is fixed in particular, conditionally on $\xi$).

Let us define the $\sigma$-fields

$$\mathcal{F}_\ell = \sigma\left((V_{\ell'},\ \ \ell \leq \ell' \leq m+n),\ \xi\right),\ \ 1 \leq \ell \leq m+n, \tag{S8}$$

where $\sigma(\cdot)$ denotes the $\sigma$-field operator. The latter form a filtration $\mathcal{F}_{m+n} \subseteq \mathcal{F}_{m+n-1} \subseteq \cdots \subseteq \mathcal{F}_1$. Note also that

$$\mathcal{F}_\ell = \sigma\left((s_{\ell'})_{\ell'\in L, \ell+1\leq \ell'\leq m+n}, V_\ell, \xi\right) = \sigma\left((s_{\ell'})_{\ell+1\leq \ell'\leq m+n}, V_\ell, \xi\right).$$

A first key point is that $\{\hat\ell \leq \ell - 1\} \in \mathcal{F}_\ell$ for all $\ell \in \{1, \ldots, m+n\}$, which means that $\hat\ell$ is a stopping time with respect to the filtration $(\mathcal{F}_\ell)_\ell$. Indeed, by (S1), we have

$$\{\hat\ell \leq \ell - 1\} = \left\{\forall \ell' \in \{\ell, \ldots, m+n\}, \frac{m}{n+1}\frac{1+V_{\ell'}}{1 \vee (\ell' - V_{\ell'})} > \alpha\right\}.$$

Hence, $\{\hat\ell \leq \ell - 1\}$ is an event measurable in $V_{\ell'}$, $\ell' \geq \ell$.

A second key point is the following lemma:

**Lemma S3.** *Consider the process $(M_\ell)_{1\leq\ell\leq m+n}$ defined by (S7) and the filtration (S8). Then $(M_{m+n}, M_{m-1}, \ldots, M_1)$ is a super-martingale with respect to the filtration $(\mathcal{F}_{m+n}, \mathcal{F}_{m+n-1}, \ldots, \mathcal{F}_1)$ (note that time is running backwards) that is, $M_\ell \in \mathcal{F}_\ell$ for all $\ell \in \{1, \ldots, m+n\}$ and*

$$\mathbb{E}(M_\ell \mid \mathcal{F}_{\ell+1}) = M_{\ell+1} - \mathbb{1}_{\{V_{\ell+1}=0, \ell+1\in L\}} \leq M_{\ell+1}, \quad 1 \leq \ell \leq m+n-1, \tag{S9}$$

*where $V_\ell$ is defined by (S3) and $L$ is given by (S2).*

Applying this lemma, we obtain

$$\begin{aligned}
\mathbb{E}[M_{\hat\ell}\mathbb{1}_{\{\hat\ell\geq 1\}} \mid \xi] &= \sum_{\ell=1}^{m+n} \mathbb{E}[M_\ell\, \mathbb{1}_{\{\hat\ell=\ell\}} \mid \xi] \\
&= \sum_{\ell=1}^{m+n} \mathbb{E}[M_\ell\, (\mathbb{1}_{\{1\leq\hat\ell\leq\ell\}} - \mathbb{1}_{\{1\leq\hat\ell\leq\ell-1\}}) \mid \xi] \\
&= \mathbb{E}[M_{m+n} \mid \xi] + \sum_{\ell=1}^{m+n-1} \mathbb{E}[(M_\ell \mathbb{1}_{\{1\leq\hat\ell\leq\ell\}} \mid \xi] - \sum_{\ell=1}^{m+n} \mathbb{E}[M_\ell \mathbb{1}_{\{1\leq\hat\ell\leq\ell-1\}} \mid \xi].
\end{aligned}$$

Hence, we obtain

$$\begin{aligned}
\mathbb{E}[M_{\hat\ell}\mathbb{1}_{\{\hat\ell\geq 1\}}\,|\,\xi] &= \mathbb{E}[M_{m+n}\,|\,\xi] + \sum_{\ell=1}^{m+n-1}\mathbb{E}[(M_\ell - M_{\ell+1})\mathbb{1}_{\{1\leq\hat\ell\leq\ell\}}\,|\,\xi]\\
&= \mathbb{E}[M_{m+n}\,|\,\xi] + \sum_{\ell=1}^{m+n-1}\mathbb{E}[\mathbb{1}_{\{1\leq\hat\ell\leq\ell\}}\mathbb{E}[(M_\ell - M_{\ell+1})\mid\mathcal{F}_{\ell+1}]\,|\,\xi]\\
&= \mathbb{E}[M_{m+n}\,|\,\xi] + \sum_{\ell=1}^{m+n-1}\mathbb{E}[\mathbb{1}_{\{1\leq\hat\ell\leq\ell\}}(\mathbb{E}[M_\ell\mid\mathcal{F}_{\ell+1}] - M_{\ell+1})\,|\,\xi]\\
&= \mathbb{E}[M_{m+n}\,|\,\xi] - \sum_{\ell=1}^{m+n-1}\mathbb{P}[1\leq\hat\ell\leq\ell, V_{\ell+1}=0, \ell+1\in L]\\
&= \mathbb{E}[M_{m+n}\,|\,\xi],
\end{aligned}$$

by using successively (S9), the fact that $\{1\leq\hat\ell\leq\ell\}\in\mathcal{F}_{\ell+1}$ and Lemma S4 (below). Now, we conclude because

$$\mathbb{E}[M_{m+n}\,|\,\xi] = \frac{\sum_{\ell\in L}(1-s_\ell)}{\sum_{\ell\in L}s_\ell + 1} = \frac{m_0}{n+1}.$$

**Lemma S4.** *For all $\ell\in\{2,\dots,m+n\}$, consider $V_\ell$ is defined by (S3), $\hat\ell$ and $\widehat{FDP}_\ell$ defined by (S1). If $V_\ell = 0$, then $\hat\ell\geq\ell$.*

*Proof.* Recall (S1) and let $\ell\in\{2,\dots,m+n\}$. If $V_\ell=0$, this implies that for any $\ell'\in\{1,\dots,\ell\}$, we have $V_{\ell'}\leq V_\ell = 0$ and thus,

$$\widehat{\mathrm{FDP}}_{\ell'} = \frac{m}{n+1}\frac{1}{\ell'}$$

because $\sum_{\ell''=1}^{\ell'}(1-s_{\ell''}) = \ell' - V_{\ell'} = \ell'$. As a result, the function $\ell'\in\{1,\dots,\ell\}\mapsto\widehat{\mathrm{FDP}}_{\ell'}$ is decreasing. This implies $\hat\ell\geq\ell$ by definition of $\hat\ell$. □

### *S1.5. Proof of Lemma S3*

Recall

$$M_\ell = \frac{\sum_{\ell'\in L,1\leq\ell'\leq\ell}(1-s_{\ell'})}{\sum_{\ell'\in L,1\leq\ell'\leq\ell}s_{\ell'}+1} = \frac{m_{0,\ell}-V_\ell}{V_\ell+1}, 1\leq\ell\leq m+n,$$

and let us prove (S9). Let $1\leq\ell\leq m+n-1$. For $\ell+1\notin L$, we have $M_\ell = M_{\ell+1}$ so (S9) holds true. Assume thus $\ell+1\in L$. We have in that case

$$\begin{aligned}
M_\ell &= \frac{m_{0,\ell}-V_\ell}{V_\ell+1}\\
&= \frac{m_{0,\ell+1}+s_{\ell+1}-1-V_{\ell+1}}{V_{\ell+1}-s_{\ell+1}+1}.
\end{aligned}$$

because $m_{0,\ell+1} = m_{0,\ell}+1$. Remember $\mathcal{F}_\ell = \sigma\left((s_{\ell'})_{\ell+1\leq\ell'\leq m+n,\ell'\in L}, V_\ell, \xi\right)$. We should now study the distribution of $s_{\ell+1}$ conditionally on $(s_{\ell'})_{\ell+2\leq\ell'\leq m+n}, V_\ell, \xi$. Remember that $S=\{\ell\in L:s_\ell = 1\}$ is uniformly distributed among all subset of $L$ of cardinality $n$, conditionally on $\xi$. Hence, by applying Lemma S2 below (with $q=n+m_0$, $u=m_{0,\ell}$ and $\{1,\dots,q\}$ in place of $L$), we obtain

$$\mathbb{P}\left(s_{\ell+1}=1\;\middle|\;(s_{\ell'})_{\ell+2\leq\ell'\leq m+n,\ell'\in L}, V_{\ell+1},\xi\right) = V_{\ell+1}/m_{0,\ell+1}.$$

This gives for $V_{\ell+1} \geq 1$,

$$\begin{aligned}\mathbb{E}(M_\ell \mid \mathcal{F}_{\ell+1}) &= \frac{V_{\ell+1}}{m_{0,\ell+1}} \frac{m_{0,\ell+1} - V_{\ell+1}}{V_{\ell+1}} + \frac{m_{0,\ell+1} - V_{\ell+1}}{m_{0,\ell+1}} \frac{m_{0,\ell+1} - 1 - V_{\ell+1}}{V_{\ell+1} + 1} \\ &= \frac{m_{0,\ell+1} - V_{\ell+1}}{m_{0,\ell+1}} \left(1 + \frac{m_{0,\ell+1} - 1 - V_{\ell+1}}{V_{\ell+1} + 1}\right) \\ &= \frac{m_{0,\ell+1} - V_{\ell+1}}{V_{\ell+1} + 1} = M_{\ell+1}.\end{aligned}$$

The last thing to check is that if $V_{\ell+1} = 0$ then $M_\ell = m_{0,\ell+1} - 1$ and $M_{\ell+1} = m_{0,\ell+1}$, so that $\mathbb{E}(M_\ell \mid \mathcal{F}_{\ell+1}) = M_{\ell+1} - 1$. This gives (S9) for any possible value of $V_{\ell+1}$.

## S2. Proofs for power results

### *S2.1. Proof of Proposition 4.1*

Recall that for the oracle $p$-values $p_i = F_0(X_i)$, $1 \leq i \leq m$ sorted as $p_{(0)} = 0 \leq p_{(1)} \leq \cdots \leq p_{(m)}$, the oracle BH procedure at level $\alpha$ is defined by

$$\mathrm{BH}^*_\alpha = \{i \in \{1, \ldots, m\} \,:\, p_i \leq p_{(k^*)}\}, \;\; k^* = \max\{k \in \{0, 1, \ldots, m\} \,:\, p_{(k)} \leq \alpha k/m\}.$$

or, equivalently,

$$\mathrm{BH}^*_\alpha = \{i \in \{1, \ldots, m\} \,:\, X_i \geq X_{(k^*)}\}, \;\; k^* = \max\{k \in \{0, 1, \ldots, m\} \,:\, X_{(k)} \geq F_0^{-1}(\alpha k/m)\}.$$

The $\hat{p}$-values are $\widehat{p}_i = \widehat{F}_0(X_i)$, $1 \leq i \leq m$, where $\widehat{F}_0$ is defined by (6), and the semi-supervised BH procedure at level $\alpha(1 + \eta)$ is given by

$$\widehat{\mathrm{BH}}_{\alpha(1+\eta)} = \{i \in \{1, \ldots, m\} \,:\, \widehat{F}_0(X_i) \leq \widehat{F}_0(X_{(\hat{k})})\},$$

with $\widehat{k} = \max\{k \in \{0, 1, \ldots, m\} \,:\, \widehat{F}_0(X_{(k)}) \leq \alpha(1 + \eta)k/m\}$. Hence, since $\widehat{F}_0$ is non-increasing, we have that $X_i \geq X_{(k^*)}$ implies $\hat{F}_0(X_i) \leq \hat{F}_0(X_{(k^*)})$, hence

$$\mathrm{BH}^*_\alpha \subseteq \{i \in \{1, \ldots, m\} \,:\, \widehat{F}_0(X_i) \leq \widehat{F}_0(X_{(k^*)})\}$$

which is itself contained in $\widehat{\mathrm{BH}}_{\alpha(1+\eta)}$ provided that $k^* \leq \widehat{k}$. By definition of $\widehat{k}$, the latter holds true whenever

$$\widehat{F}_0(X_{(k^*)}) \leq \alpha(1 + \eta)k^*/m. \tag{S10}$$

Since $X_{(k^*)} \geq F_0^{-1}(\alpha k^*/m)$, we have $\widehat{F}_0(X_{(k^*)}) \leq \widehat{F}_0(F_0^{-1}(\alpha k^*/m))$ and (S10) holds if $\widehat{F}_0(F_0^{-1}(\alpha k^*/m)) \leq \alpha(1 + \eta)k^*/m$. To sum up, we obtained that

$$\mathbb{P}(\mathrm{BH}^*_\alpha \subseteq \widehat{\mathrm{BH}}_{\alpha(1+\eta)}) \geq \mathbb{P}(\Omega)$$

with $\Omega = \{\widehat{F}_0(F_0^{-1}(\alpha k^*/m)) \leq \alpha(1 + \eta)k^*/m\}$.

Now, let us upper bound the probability of $\Omega^c$ as follows: assume first

$$\eta^2 \alpha\gamma \geq \frac{28}{3} \log 2. \tag{S11}$$

Letting $u_k = F_0^{-1}(\alpha k/m)$, and $\widetilde{F}_0(x) = n^{-1} \sum_{j=1}^n \mathbb{1}_{\{Y_j \geq x\}} = \frac{n+1}{n} \widehat{F}_0(x) - 1/n$, see (6), (so that $\mathbb{E}\widetilde{F}_0(x) = F_0(x)$), we have $\mathbb{P}(\Omega^c) = \mathbb{P}(\Omega^c, k^* > 0)$ with

$$\begin{aligned}\mathbb{P}(\Omega^c, k^*>0) &\leq \sum_{k=1}^m \mathbb{P}(\widehat{F}_0(u_k) > \alpha(1+\eta)k/m) = \sum_{k=1}^m \mathbb{P}\left(\widetilde{F}_0(u_k) > \frac{(n+1)\alpha(1+\eta)k/m - 1}{n}\right)\\ &\leq \sum_{k=1}^m \mathbb{P}\left(\widetilde{F}_0(u_k) > \alpha(1+\eta)k/m - 1/n\right) = \sum_{k=1}^m \mathbb{P}(n(\widetilde{F}_0 - F_0)(u_k) > \alpha\eta kn/m - 1)\\ &\leq \sum_{k=1}^m \mathbb{P}(n(\widetilde{F}_0 - F_0)(u_k) > 0.5\alpha\eta kn/m),\end{aligned}$$

by noting that $F_0(u_k) = \alpha k/m$ and that $a = \eta\alpha kn/m$ satisfies $a - 1 \geq 0.5a$ because $a \geq 2$, by using (S11). Indeed, $a = \eta\alpha kn/m \geq \eta^2\alpha n/m \geq \eta^2\alpha\gamma \geq \frac{28}{3}\log 2 \geq 2$. Applying Bernstein's inequality (Lemma S1 with $W_i = \mathbb{1}_{\{Y_i \geq u_k\}}$, $\mathcal{M} = 1$, $V = \alpha kn/m$, $A = 0.5\alpha\eta kn/m$), we obtain

$$\begin{aligned}\mathbb{P}(\Omega^c) &\leq \sum_{k=1}^m \exp\left\{-\frac{(0.5\alpha\eta kn/m)^2}{2\alpha kn/m + 2(0.5\alpha\eta kn/m)/3)}\right\}\\ &\leq \sum_{k=1}^m \exp\left\{-\frac{3}{28}\eta^2\alpha kn/m\right\} \leq \frac{e^{-z}}{1-e^{-z}} \leq 2e^{-z},\end{aligned}$$

for $z = \frac{3}{28}\eta^2\alpha n/m$, which is such that $z \geq \log 2$ by (S11).

Summing up, we have proved that for any $\alpha, \eta \in (0,1)$ with $\eta^2\alpha\gamma \geq \frac{28}{3}\log 2$,

$$\mathbb{P}_{Z\sim P}(\mathrm{BH}^*_\alpha \subseteq \widehat{\mathrm{BH}}_{\alpha(1+\eta)}) \geq 1 - 2\exp(-(3/28)\alpha\eta^2\gamma).$$

Applying this for $\alpha' = \alpha/(1+\eta) \in (0,1)$ in place of $\alpha$, we obtain that for all $\alpha, \eta \in (0,1)$ with $\eta^2\alpha\gamma \geq (1+\eta)\frac{28}{3}\log 2$,

$$\mathbb{P}_{Z\sim P}(\mathrm{BH}^*_{\alpha'} \subseteq \widehat{\mathrm{BH}}_\alpha) \geq 1 - 2\exp(-(3/28)\alpha(1+\eta)^{-1}\eta^2\gamma).$$

Since $\mathrm{BH}^*_{\alpha(1-\eta)} \subseteq \mathrm{BH}^*_{\alpha'}$ because $1-\eta \leq 1/(1+\eta)$, we obtain

$$\mathbb{P}_{Z\sim P}(\mathrm{BH}^*_{\alpha(1-\eta)} \subseteq \widehat{\mathrm{BH}}_\alpha) \geq 1 - 2\exp(-(3/28)\alpha\gamma\eta^2/(1+\eta)).$$

Also, we note that this bound is also true (and trivial) when $\eta^2\alpha\gamma < (1+\eta)\frac{28}{3}\log 2$. We obtain finally the result by plugging $\gamma_*(\alpha,\eta)$ into the bound.

### *S2.2. Proof of Proposition 4.2*

We start by proving the following result.

**Lemma S1.** *Assume (Indep) and let $\alpha \in (0,1)$ and $n, m \geq 1$. Then for any $P \in \mathcal{A}_{n,m}$, we have that $2\alpha m_1(P) \leq m/(n+1)$ implies*

$$\mathbb{P}_{Z\sim P}(TDP(P, \widehat{BH}_\alpha) = 0) \geq 1 - 2\alpha. \tag{S12}$$

*In particular, if $(n+1)/m \leq 1/(2\alpha)$, inequality (S12) holds for all $P \in \mathcal{A}_{n,m}$ with $m_1(P) = 1$.*

Before proving Lemma S1, let us show that it implies Proposition 4.2. For this, let us consider $\alpha \in (0, 1/4)$, $\eta \in (0,1)$ and $n, m \geq 1$ with $n/m \leq 1/(4\alpha)$. Then we have $(n+1)/m \leq 1/(4\alpha) + 1/m \leq 1/(2\alpha)$. Applying (S12) for $P_a = \mathcal{N}(0,1)^{\otimes(n+m-1)} \otimes \mathcal{N}(a,1)$ (note $m_1(P_a) = 1$), we have for all $a > 0$,

$$\mathbb{P}_{Z\sim P_a}(\mathrm{TDP}(P, \widehat{\mathrm{BH}}_\alpha) = 0) \geq 1 - 2\alpha.$$

Now, we have that $\mathrm{BH}^*_{\alpha(1-\eta)}$ rejects the only null hypotheses that is false for $P_a$ provided that $\bar\Phi(X_m) \leq \alpha(1-\eta)/m$, where $\bar\Phi$ denotes the standard Gaussian upper tail function. This occurs with probability $\bar\Phi(\bar\Phi^{-1}(\alpha(1-\eta)/m) - a)$. Therefore, for all $a > 0$,

$$\mathbb{P}_{Z\sim P_a}(\mathrm{TDP}(P, \widehat{\mathrm{BH}}_\alpha) = 0, \mathrm{TDP}(P, \mathrm{BH}^*_{\alpha(1-\eta)}) > 0) \geq \bar\Phi(\bar\Phi^{-1}(\alpha(1-\eta)/m) - a) - 2\alpha.$$

This entails for all $a > 0$,

$$\sup_{P\in\mathcal{A}_{n,m}} \{\mathbb{P}_{Z\sim P}(\mathrm{TDP}(P, \widehat{\mathrm{BH}}_\alpha) < \mathrm{TDP}(P, \mathrm{BH}^*_{\alpha(1-\eta)}))\} \geq \bar\Phi(\bar\Phi^{-1}(\alpha(1-\eta)/m) - a) - 2\alpha.$$

Now making $a$ tending to infinity gives (17).

Let us now prove Lemma S1. Consider $P \in \mathcal{A}_{n,m}$. Assume $2\alpha m_1(P) \leq m/(n+1)$. Denotes $\hat k \geq 0$ the number of rejections of $\widehat{\mathrm{BH}}_\alpha$. First observe that $\hat k \geq 2m_1(P)$ implies $\mathrm{FDP}(P, \widehat{\mathrm{BH}}_\alpha) \geq (\hat k - m_1(P))/\hat k \geq 1/2$. Applying the Markov inequality, we thus derive

$$\mathbb{P}_{Z\sim P}(\hat k \geq 2m_1(P)) \leq \mathbb{P}_{Z\sim P}(\mathrm{FDP}(P, \widehat{\mathrm{BH}}_\alpha) \geq 1/2) \leq 2\,\mathrm{FDR}(P, \widehat{\mathrm{BH}}_\alpha) \leq 2\alpha,$$

because $\mathrm{FDR}(P, \widehat{\mathrm{BH}}_\alpha) \leq \alpha$ by Theorem 3.1. On the other hand, if $\hat k < 2m_1(P)$ then because $2\alpha m_1(P) \leq m/(n+1)$, we have that all $\hat p$-values are larger than or equal to (see (5))

$$1/(n+1) \geq 2\alpha m_1(P)/m > \alpha \hat k/m.$$

Hence $\hat k = 0$ by definition of the BH procedure (7). This entails $\mathrm{TDP}(P, \widehat{\mathrm{BH}}_\alpha) = 0$. Putting the above relations together, we obtain

$$\mathbb{P}_{Z\sim P}(\mathrm{TDP}(P, \widehat{\mathrm{BH}}_\alpha) > 0) \leq \mathbb{P}_{Z\sim P}(\hat k \geq 2m_1(P)) \leq 2\alpha,$$

which concludes the proof.

### *S2.3. Proof of Proposition 4.3*

Point (i) is similar to the proof of Proposition 4.1, see Section S2.1. The only difference is that we can use that the number of correct rejections of the oracle procedure is larger or equal to $k$, with large probability, because $P \in \mathcal{A}_{n,m,k,\alpha,\beta}$.

Consider $nk/m \geq \gamma$ for some $\gamma > 0$. We first prove that for $\alpha' \in (\alpha/2, 1)$, $\eta \in (0, 1/2)$, if $\eta^2\alpha'\gamma \geq \frac{28}{3}\log 2$,

$$\mathbb{P}_{Z\sim P}(\mathrm{BH}^*_\alpha \subseteq \widehat{\mathrm{BH}}_{\alpha(1+\eta)}) \geq 1 - \beta - 2\exp(-(3/28)\alpha\eta^2\gamma).$$

For this, we use exactly the same proof as in Section S2.1, except that we use $k^* \geq k$ when $k^* > 0$ on an event of probability larger than $1-\beta$ (see notation therein). Hence, we obtain

$$\mathbb{P}(\Omega^c, k^* > 0) \leq \beta + \mathbb{P}(\Omega^c, k^* \geq k) \leq \sum_{k'=k}^m e^{-k'z} \leq 2e^{-kz}.$$

$z = \frac{3}{28}\eta^2\alpha' n/m$, which proves the intermediate result above. Now, Point (i) comes by applying this with $\alpha' = \alpha/(1+\eta) \geq \alpha(1-\eta) \geq \alpha/2$ because $\eta < 1/2$.

Point (ii) is similar to the proof of Proposition 4.2, see Section S2.2. Consider any distribution $P \in \mathcal{A}_{n,m,k,\alpha,\beta}$ with $m_1(P) = k$ and

$$\mathbb{P}_{Z\sim P}(\mathrm{TDP}(P, \mathrm{BH}^*_{\alpha(1-\eta)}) = 1) \geq 1 - \beta$$

(we easily check that such a distribution exists with Gaussian alternatives with alternative mean large enough). Applying Lemma S1 with this distribution $P$, we obtain that if $2\alpha k \leq m/(n+1)$, that is, $(n+1)k/m \leq 1/(2\alpha)$,

$$\mathbb{P}_{Z\sim P}(\mathrm{TDP}(P, \widehat{\mathrm{BH}}_\alpha) = 0) \geq 1 - 2\alpha.$$

This gives Point (ii) by noting that $(n+1)k/m \leq 1/(4\alpha) + k/m \leq 1/(2\alpha)$ because $k/m \leq 1 \leq 1/(4\alpha)$.

### *S2.4. Proof of Theorem 5.1*

The proof relies on the construction of particular distributions for the $Y_i$'s and the $X_i$'s. Also remember that the BH procedure rejects for large values of $X_i$'s. For instance, if $X_i \sim U(0,1)$ under the null, any $X_i \in [1-\alpha/m, 1]$ will be in the rejection set of the oracle BH procedure at level $\alpha$.

Let $\alpha' = \alpha(1-\eta)$. For some constant $\kappa > 0$ with $\kappa/n < 1$ (to be chosen later on), let us consider the two following distribution on $\mathbb{R}$

$$\mu = (1-\kappa/n)\, U(0,1) + (\kappa/n)\, U(1-\alpha'/m, 1) \tag{S13}$$

and the following distributions on $\mathbb{R}^{n+m}$

$$Q_1 = \mu^{\otimes(n+m)},\ \ Q_{2,u} = U(0,1)^{\otimes n} \otimes \bigotimes_{i=1}^{m} \left((1-u_i)U(0,1) + u_i U(1-\alpha'/m, 1)\right),\ \ u \in \mathbb{R}^m. \tag{S14}$$

Observe that $\mathcal{H}_0(Q_1) = \{1,\dots,m\}$, $m_0(Q_1) = m$, $\mathcal{H}_0(Q_{2,u}) = \{i \in \{1,\dots,m\} \ :\ u_i = 0\}$, $m_0(Q_{2,u}) = \sum_{i=1}^m (1-u_i)$, for all $u \in \mathbb{R}^m$. Now consider $U_i$, $1 \le i \le m$, that are i.i.d. $\mathcal{B}(\kappa/n)$ and $U = (U_i)_{1\le i \le n}$. Then any $Z \sim Q_{2,U}$ is distributed as $Q_2 = U(0,1)^{\otimes n} \otimes \mu^{\otimes m}$ unconditionally on $U$.

For any procedure $R = R(Z)$, we have $\mathrm{FDR}(Q_1, R) = \mathbb{P}_{Z\sim Q_1}(|R| > 0)$ (remember $\mathcal{H}_0(Q_1) = \{1,\dots,m\}$). Since $\mathbb{P}_{Z\sim Q_1}(|R| > 0) + \mathbb{P}_{Z\sim Q_1}(|R| = 0) = 1$. Either $\mathrm{FDR}(Q_1, R) = \mathbb{P}_{Z\sim Q_1}(|R| > 0) \ge 1/2$, or $\mathbb{P}_{Z\sim Q_1}(|R| = 0) \ge 1/2$, in which case $\mathbb{P}_{Z\sim Q_2}(|R| = 0) \ge 1/2 - d_{tv}(Q_1, Q_2)$, where $d_{tv}(Q_1,Q_2) = \sup_{\mathcal{A}} |Q_1(A) - Q_2(A)|$ denotes the total variation distance between the distributions $Q_1$ and $Q_2$. Hence, in the latter case, we obtain (recall the definition of the $U_i$'s above)

$$\begin{aligned}
1/2 - d_{tv}(Q_1,Q_2) &\le \mathbb{E}_U \mathbb{P}_{Z\sim Q_{2,U}}(|R(Z)| = 0)\\
&\le \mathbb{E}_U \left(\mathbb{1}_{\{\sum_{i=1}^m U_i \ge 1\}} \mathbb{P}_{Z\sim Q_{2,U}}(|R(Z)| = 0)\right) + \mathbb{P}_U\left(\sum_{i=1}^m U_i = 0\right)\\
&\le \mathbb{E}_U \left(\mathbb{1}_{\{\sum_{i=1}^m U_i \ge 1\}} \mathbb{P}_{Z\sim Q_{2,U}}(|R(Z)| = 0)\right) + (1-\kappa/n)^m\\
&\le \mathbb{E}_U \left(\mathbb{1}_{\{\sum_{i=1}^m U_i \ge 1\}} \mathbb{P}_{Z\sim Q_{2,U}}(|R(Z)| = 0, |\mathrm{BH}^*_{\alpha'} \cap \mathcal{H}_1(Q_{2,U})| \ge 1)\right) + e^{-\kappa m/n},
\end{aligned}$$

because by definition of $Q_{2,U}$ the null hypothesis corresponding to any index $i$ with $U_i = 1$ corresponds to a $X_i$ larger than $1-\alpha'/m$ and thus is rejected by $\mathrm{BH}^*_{\alpha'}$. Note that we also used $(1-\kappa/n)^m \le e^{-\kappa m/n}$ because for all $u \in [0,1)$, $\log(1-u) \le -u$. The last display entails that

$$\sup_{u\in\mathbb{R}^m} \left\{\mathbb{P}_{Z\sim Q_{2,u}}(|R(Z)| = 0, |\mathrm{BH}^*_{\alpha'} \cap \mathcal{H}_1(Q_{2,u})| \ge 1)\right\} \ge 1/2 - e^{-\kappa m/n} - d_{tv}(Q_1,Q_2).$$

Summing up, we obtained that for any procedure $R$, either $\mathrm{FDR}(Q_1,R) \ge 1/2$, or there exist some distribution $Q_{2,u}$, $u \in \mathbb{R}^m$, with $m_1(Q_{2,u}) \ge 1$ and

$$\mathbb{P}_{Z\sim Q_{2,u}}\left(\mathrm{FDP}(R, Q_{2,u}) < \mathrm{FDP}(\mathrm{BH}^*_{\alpha'/2}, Q_{2,u})\right) \ge 1/2 - e^{-\kappa m/n} - d_{tv}(Q_1,Q_2).$$

It only remains to upper bound the total variation distance $d_{tv}(Q_1,Q_2)$. From Le Cam's inequalities and tensorization identities for Hellinger distances, see, e.g., Tsybakov (2009) Section 2.4, we have that

$$\begin{aligned}
d_{tv}(Q_1,Q_2)^2 &\le \int_{\mathbb{R}^n}\int_{\mathbb{R}^m} \left(\prod_{i=1}^n f_\mu^{1/2}(y_i) \prod_{i=1}^m f_\mu^{1/2}(x_i) - \prod_{i=1}^n g^{1/2}(y_i) \prod_{i=1}^m f_\mu^{1/2}(x_i)\right)^2 dxdy\\
&= \int_{\mathbb{R}^n} \left(\prod_{i=1}^n f_\mu^{1/2}(y_i) - \prod_{i=1}^n g^{1/2}(y_i)\right)^2 dy \le n \int_{\mathbb{R}} \left(f_\mu^{1/2}(y) - g^{1/2}(y)\right)^2 dy,
\end{aligned}$$

where $f_\mu(y) = (1-\kappa/n)\mathbb{1}_{\{y\in[0,1]\}} + \frac{\kappa m}{n\alpha'}\mathbb{1}_{\{y\in[1-\alpha'/m,1]\}}$, $y \in \mathbb{R}$, denotes the density of $\mu$, while $g(y) = \mathbb{1}_{\{y\in[0,1]\}}$, $y\in\mathbb{R}$, denotes the density of $U(0,1)$. Now, we have

$$d_{tv}(Q_1,Q_2)^2 \le n\int_{1-\alpha'/m}^1 \left(\left(\frac{\kappa m}{n\alpha'}+1-\kappa/n\right)^{1/2}-1\right)^2 dy + n\int_0^{1-\alpha'/m}\left(1-(1-\kappa/n)^{1/2}\right)^2 dy$$
$$= \frac{n\alpha'}{m}\left(\left(\frac{\kappa m}{n\alpha'}+1-\kappa/n\right)^{1/2}-1\right)^2 + n\left(1-(1-\kappa/n)^{1/2}\right)^2.$$

Now note that $1 \le \frac{\kappa m}{n\alpha'} + 1 - \kappa/n \le \frac{\kappa m}{n\alpha'}+1$, which entails

$$\left(\left(\frac{\kappa m}{n\alpha'}+1-\kappa/n\right)^{1/2}-1\right)^2 \le \left(\left(1+\frac{\kappa m}{n\alpha'}\right)^{1/2}-1\right)^2 \le \left(\frac{\kappa m}{2n\alpha'}\right)^2$$

where we used that for all $u\ge 0$, $(1+u)^{1/2}-1\le u/2$. Furthermore, for all $u\in[0,1]$, $1-(1-u)^{1/2}\le u$ and thus $\left(1-(1-\kappa/n)^{1/2}\right)^2 \le (\kappa/n)^2$. Hence, we obtain (since $m\ge 4\alpha'$),

$$d_{tv}(Q_1,Q_2)^2 \le \frac{n\alpha'}{m}\left(\frac{\kappa m}{2n\alpha'}\right)^2 + n(\kappa/n)^2 = (\kappa^2/n)\left(\frac{m}{4\alpha'}+1\right) \le \kappa^2\frac{m}{2n\alpha'}.$$

Now, to make $e^{-\kappa m/n} + \kappa\sqrt{\frac{m}{2n\alpha'}}$ small, we can choose $\kappa = (n/m)\log(1+m/n)$, to get the bound $\frac{n}{m} + \sqrt{\frac{n\log(1+m/n)}{2m\alpha'}} \le \gamma + \sqrt{\frac{\gamma\log(1+\gamma^{-1})}{2\alpha(1-\eta)}}$, because $\log(1+m/n)\ge\log(2)\ge 1$ $n/m\ge\gamma$ and $h(u) = u\log(1+1/u)$ is increasing on $\mathbb{R}_+$ (for instance, we have $h''(u) = -1/(u(u+1)^2)$ and $h'(10)>0$). We also check that $\kappa/n<1$, which holds because $\gamma\log(1+\gamma^{-1})\le\log(2)<1\le n$.

Finally, we obtained that for any procedure $R$, either (17) holds or

$$\sup_{P\in\mathcal{A}_{n,m}}\{\mathbb{P}_{Z\sim P}(\mathrm{TDP}(P,R) < \mathrm{TDP}(P,\mathrm{BH}^*_{\alpha(1-\eta)}))\} \ge 1/2 - \gamma - \sqrt{\frac{\gamma\log(1+\gamma^{-1})}{2\alpha(1-\eta)}} \quad \text{(S15)}$$

holds. Since for all $x>1$, we have $x^{-1/3}\log(1+x)\le 2$, this entails

$$\gamma + \sqrt{\frac{\gamma\log(1+\gamma^{-1})}{2\alpha(1-\eta)}} \le \gamma^{1/3}(1+(\alpha(1-\eta))^{-1/2}) = (\gamma/(64\gamma_*(\alpha,\eta)))^{1/3},$$

bu definition of $\gamma_*(\alpha,\eta)$. This gives the main statement. Let us now prove the additional statement. Choose any sequence $\gamma_k\in\mathbb{Q}$ with $0<\gamma_k\le\gamma$ and $\gamma_k\to\gamma$ when $k\to\infty$. Since $\gamma_k$ is of the form $n/m$ with $n,m\ge 1$ being two integers, the previous statement applied with $n = m\gamma_k$ shows that

$$\max\Bigg(\sup_{\substack{n,m\ge 1\\ n\ge m\gamma_k}}\sup_{P\in\mathcal{P}_{n,m}}\{\mathrm{FDR}(P,R)-\mathrm{FDR}(\mathrm{BH}^*_\alpha,R)\} - (1/2-\alpha),$$
$$\sup_{\substack{n,m\ge 1\\ n\ge m\gamma_k}}\sup_{P\in\mathcal{A}_{n,m}}\{\mathbb{P}(\mathrm{TDP}(P,\mathrm{BH}^*_{\alpha(1-\eta)}) > \mathrm{TDP}(P,R)\} - 1/2 - (\gamma_k/(8\gamma_*(\alpha,\eta)))^{1/3}\Bigg) \ge 0$$

Hence, we also have

$$\max\Bigg(\sup_{\substack{n,m\ge 1\\ n\ge m\gamma}}\sup_{P\in\mathcal{P}_{n,m}}\{\mathrm{FDR}(P,R)-\mathrm{FDR}(\mathrm{BH}^*_\alpha,R)\} - (1/2-\alpha),$$
$$\sup_{\substack{n,m\ge 1\\ n\ge m\gamma}}\sup_{P\in\mathcal{A}_{n,m}}\{\mathbb{P}(\mathrm{TDP}(P,\mathrm{BH}^*_{\alpha(1-\eta)}) > \mathrm{TDP}(P,R)\} - 1/2 - (\gamma_k/(8\gamma_*(\alpha,\eta)))^{1/3}\Bigg) \ge 0.$$

Making $k$ tending to infinity, we get

$$\max\left(\sup_{\substack{n,m\geq 1\\ n\geq m\gamma}}\sup_{P\in\mathcal{P}_{n,m}}\{\mathrm{FDR}(P,R)-\mathrm{FDR}(\mathrm{BH}^*_\alpha,R)\}-(1/2-\alpha),\right.$$

$$\left.\sup_{\substack{n,m\geq 1\\ n\geq m\gamma}}\sup_{P\in\mathcal{A}_{n,m}}\{\mathbb{P}(\mathrm{TDP}(P,\mathrm{BH}^*_{\alpha(1-\eta)})>\mathrm{TDP}(P,R)\}-1/2-(\gamma/(8\gamma_*(\alpha,\eta)))^{1/3}\right)\geq 0.$$

This excludes that (14) and (15) simultaneously holds for $\delta_1<1/2-\alpha$ and $\delta_2<1/2-(\gamma/(8\gamma_*(\alpha,\eta)))^{1/3}$.

## S3. Auxiliary results

**Lemma S1.** *[Bernstein's inequality] Let $W_i$, $1\leq i\leq n$ centered independent variables with $|W_i|\leq\mathcal{M}$ and $\sum_{i=1}^n\mathrm{Var}(W_i)\leq V$, then for any $A>0$,*

$$P\left[\sum_{i=1}^n W_i>A\right]\leq\exp\left\{-\frac{1}{2}A^2/(V+\mathcal{M}A/3)\right\}.$$

**Lemma S2.** *Let $\varepsilon_1,\dots,\varepsilon_q\in\{0,1\}$ be exchangeable binary random variables, $1\leq u\leq q$, and $V=\sum_{i=1}^u\varepsilon_i$, then*

$$\mathbb{P}(\varepsilon_u=1\mid V,\varepsilon_q,\dots,\varepsilon_{u+1})=V/u.$$

*In particular, this holds if the set $\{1\leq i\leq q:\varepsilon_i=1\}$ is uniformly distributed among the subsets of $\{1,\dots,q\}$ of size $n$, for some $1\leq n\leq q$.*

Note that the following stronger result holds: conditionally on $V$ and $\varepsilon_q,\dots,\varepsilon_{u+1}$, the set $\{1\leq i\leq u:\varepsilon_i=1\}$ is uniformly distributed among the subsets of $\{1,\dots,u\}$ of size $n-V$.

*Proof.* Let us first observe that $(\varepsilon_u,\dots,\varepsilon_1)$ are exchangeable conditionally on $\sum_{i=1}^u\varepsilon_i,\varepsilon_q,\dots,\varepsilon_{u+1}$. Indeed, for any permutation $g$ of $\{1,\dots,u\}$, we have that

$$(\varepsilon_{g(u)},\dots,\varepsilon_{g(1)},\varepsilon_q,\dots,\varepsilon_{u+1})\sim(\varepsilon_u,\dots,\varepsilon_1,\varepsilon_q,\dots,\varepsilon_{u+1})$$

and since $\sum_{i=1}^u\varepsilon_i=\sum_{i=1}^u\varepsilon_{g(i)}$, we have thus

$$(\varepsilon_{g(u)},\dots,\varepsilon_{g(1)},\sum_{i=1}^u\varepsilon_i,\varepsilon_q,\dots,\varepsilon_{u+1})\sim(\varepsilon_u,\dots,\varepsilon_1,\sum_{i=1}^u\varepsilon_i,\varepsilon_q,\dots,\varepsilon_{u+1}),$$

which entails the first observation.

Hence, we have

$$V=\sum_{i=1}^u\mathbb{P}(\varepsilon_i=1\mid V,\varepsilon_q,\dots,\varepsilon_{u+1})=u\,\mathbb{P}(\varepsilon_u=1\mid V,\varepsilon_q,\dots,\varepsilon_{u+1}),$$

which gives the result. □

**Proposition S3.** *Let $k\geq 1$ and consider $(X_1,\dots,X_k)$ a $k$-dimensional centered Gaussian vector with individual variance 1 and equi-correlation $\rho\in[-1/k,1]$. Let*

$$X_{k+1}=a(X_1+\dots+X_k)+bU,\ \ a=\frac{\rho}{1+(k-1)\rho},\ \ b=(1-ak\rho)^{1/2},$$

*where $U\sim\mathcal{N}(0,1)$ is independent of $X_1,\dots,X_k$. Then the vector $(X_1,\dots,X_k,X_{k+1})$ is a $(k+1)$-dimensional centered Gaussian vector with individual variance 1 and equi-correlation $\rho$.*

As an illustration, in the extremal case $\rho = -1/k$, we have $a = -1$, $b = 0$ and $X_{k+1} = -(X_1 + \cdots + X_k)$. The opposite extremal case is $\rho = 1$, for which $a = 1/k$, $b = 0$. More generally, when $\rho \in [-1/k, 1]$, $a$ is increasing in $\rho$ from $-1$ ($\rho = -1/k$) to $1/k$ ($\rho = 1$) and we can check that $b$ is well defined because $|ak\rho| \leq 1$: when $\rho \leq 0$, $|ak\rho| \leq |a| \leq 1$ and when $\rho \geq 0$, $|ak\rho| \leq |ak| \leq 1$.

*Proof.* Since the vector $(X_1, \dots, X_k, U)$ is Gaussian, so is $(X_1, \dots, X_k, X_{k+1})$ and we just have to check that $\mathrm{Var}(X_{k+1}) = 1$ and for all $i \in \{1, \dots, k\}$, $\mathrm{Cov}(X_i, X_{k+1}) = \rho$. This comes from

$$\begin{aligned}\mathrm{Var}(X_{k+1}) &= a^2 \,\mathrm{Var}(X_1 + \cdots + X_k) + b^2\\ &= a^2(k + k(k-1)\rho) + b^2\\ &= a\frac{\rho}{1+(k-1)\rho}k(1+(k-1)\rho) + 1 - ak\rho = 1,\end{aligned}$$

and, for all $i \in \{1, \dots, k\}$,

$$\mathrm{Cov}(X_i, X_{k+1}) = a\left(1 + \sum_{1\leq j\leq k, j\neq i} \mathrm{Cov}(X_i, X_j)\right) = a(1 + (k-1)\rho) = \rho.$$

□

**Proposition S4.** *Let $\alpha \in (0,1)$ and $n, m \geq 1$ such that $\alpha(n+1)/m$ is an integer. Then if $\hat{\ell}$ given by (S1) exists, we have $\widehat{FDP}_{\hat{\ell}} = \alpha$*

*Proof.* Recall

$$\widehat{\mathrm{FDP}}_\ell = \frac{m}{n+1}\frac{1 + \sum_{\ell'=1}^{\ell} s_{\ell'}}{1 \vee \sum_{\ell'=1}^{\ell}(1 - s_{\ell'})}, \quad 1 \leq \ell \leq n+m.$$

Let $\mathcal{L} = \left\{\ell \in \{1, \dots, n+m\} \,:\, \widehat{\mathrm{FDP}}_\ell \leq \alpha\right\}$ and $\mathcal{L}' = \left\{\ell \in \{1, \dots, n+m\} \,:\, \widehat{\mathrm{FDP}}_\ell < \alpha\right\}$. By assumption, $\mathcal{L} \neq \emptyset$ and $\hat{\ell} = \max \mathcal{L}$. If $\mathcal{L}' = \emptyset$, then necessarily $\hat{\ell} \notin \mathcal{L}'$ which means $\widehat{\mathrm{FDP}}_{\hat{\ell}} = \alpha$. So we assume in the sequel $\mathcal{L}' \neq \emptyset$ and consider $\tilde{\ell} = \max \mathcal{L}' \leq \hat{\ell}$.

Let us prove $\widehat{\mathrm{FDP}}_{\tilde{\ell}+1} = \alpha$. First note that $\tilde{\ell} \leq n+m-1$ because $\widehat{\mathrm{FDP}}_{n+m-1} = 1$. In addition, we have by definition $\widehat{\mathrm{FDP}}_{\tilde{\ell}+1} \geq \alpha$, which means that $s_{\hat{\ell}+1} = 1$. Let $v = 1 + \sum_{\ell'=1}^{\tilde{\ell}+1} s_{\ell'}$, $k = 1 \vee \sum_{\ell'=1}^{\tilde{\ell}+1}(1 - s_{\ell'})$ and $a = \alpha(n+1)/m$, so that $\frac{n+1}{m}\widehat{\mathrm{FDP}}_{\tilde{\ell}+1} = v/k \geq a$ and $\frac{n+1}{m}\widehat{\mathrm{FDP}}_{\tilde{\ell}} = (v-1)/k < a$. But since $v, k$ and $a$ (by assumption) are integers, we have that $v - 1 < ak$ implies $v \leq ak$ and thus we obtain $v = ak$. This gives $\widehat{\mathrm{FDP}}_{\tilde{\ell}+1} = \frac{m}{n+1}v/k = \alpha$.

Now, since $\widehat{\mathrm{FDP}}_{\tilde{\ell}+1} \leq \alpha$ we have $\hat{\ell} \geq \tilde{\ell} + 1$. But by definition of $\tilde{\ell}$, this implies $\widehat{\mathrm{FDP}}_{\hat{\ell}} \geq \alpha$. Since $\widehat{\mathrm{FDP}}_{\hat{\ell}} \leq \alpha$ also holds, this gives $\widehat{\mathrm{FDP}}_{\hat{\ell}} = \alpha$. □

**Proposition S5.** *Let $\alpha \in (0,1)$ and $n, m \geq 1$. Then if $\hat{\ell}$ given by (S1) exists, we have $\widehat{FDP}_{\hat{\ell}} \geq \frac{m}{n+1}\lfloor \alpha\frac{n+1}{m} \rfloor$.*

*Proof.* Let $\alpha' = \frac{m}{n+1}\lfloor \alpha\frac{n+1}{m} \rfloor \leq \alpha$ and $\mathcal{L}' = \left\{\ell \in \{1, \dots, n+m\} \,:\, \widehat{\mathrm{FDP}}_\ell \leq \alpha'\right\}$. If this set is empty, this means $\widehat{\mathrm{FDP}}_{\hat{\ell}} > \alpha'$ and the conclusion holds. If this set is not empty, we can consider its maximum $\widetilde{\ell} = \max \mathcal{L}'$. Obviously, we have $\widetilde{\ell} \leq \hat{\ell}$. If $\widetilde{\ell} = \hat{\ell}$, then by Lemma S4 (since $\alpha'(n+1)/m$ is an integer), we have $\widehat{\mathrm{FDP}}_{\widetilde{\ell}} = \alpha'$, and thus also $\widehat{\mathrm{FDP}}_{\hat{\ell}} = \alpha'$ and the conclusion holds. If $\widetilde{\ell} < \hat{\ell}$, we have $\widehat{\mathrm{FDP}}_{\hat{\ell}} > \alpha'$ because $\widetilde{\ell}$ is a maximum. This shows $\widehat{\mathrm{FDP}}_{\hat{\ell}} \geq \alpha'$ in any case and proves the result. □

## S4. Additional numerical experiments

### S4.1. Comparison to naive procedures

Figure S1 shows a comparison with the two naive procedures defined in Section 1.3 for $\alpha = 0.2$ and $m = 10$ as a function of $n$. The plots display the FDR and TDR results for $\mathrm{BH}^*$ (dark green and khaki), $\widehat{\mathrm{BH}}$ (dark blue and cyan), $\widehat{\mathrm{BY}}$ (red and magenta) and $\widehat{\mathrm{BH}}_{\mathrm{Split}}$ (gray-blue and black). The left column corresponds to i.i.d. samples and the right column to equicorrelated Gaussian samples (see Section 6.2). We note immediately very similar performances in the i.i.d. and correlated cases because the considered values of $n$ are large. Under the "full null' (top row), the dense (middle row) and sparse (bottom row) cases, the convergence of the FDR is clearly much slower for the naive approaches than for $\mathrm{BH}^*$ and $\widehat{\mathrm{BH}}$. The same effect is true for the TDR in the signal-present cases. As expected, the $\widehat{\mathrm{BY}}$ approach is overly conservative to force the FDR control, which leads to a substantial loss in power. The $\widehat{\mathrm{BH}}_{\mathrm{Split}}$ approach indeed controls the FDR but also suffers from power loss at fixed $n$ with respect to the proposed $\widehat{\mathrm{BH}}$ procedure. Note that for $\widehat{\mathrm{BH}}_{\mathrm{Split}}$, the rule of thumb $nk \asymp m/\alpha$ found in Section 4 is expected to become $nk \asymp m^2/\alpha$, because the splitting process uses a training sample of length $n/m$ instead of $m$. This is what we observe in the middle and lower panels, where values of $k = 1$ and $k \approx 3$ respectively lead to $n = 500$ and $n \approx 170$. In contrast, the corresponding values of $n$ are 10 times smaller for $\widehat{\mathrm{BH}}$, which is consequently much more powerful at fixed $n$ than the naive approaches considered here.

### S4.2. Results in a non Gaussian case

Figure S2 illustrates the FDR and TDR in the case where the null distribution $P_0$ is a Student distribution with zero mean and $\nu = 3$ degrees of freedom, rescaled to have unit variance. Comparing with the Gaussian case of (Figure 5), where all other simulation parameters are the same, very similar conclusions can be drawn. In particular, the FDR control of $\widehat{\mathrm{BH}}$ indeed holds also in the case of a heavy tailed distribution since our results are distribution free. Note finally that while the power is larger in the Student case than in the Gaussian case in this setting, the situation can be reversed for other couples $(\alpha, \mu)$. As $\nu$ increases however, the powers in the Gaussian and standardized Student cases become indeed similar, and hardly distinguishable when $\nu$ reaches $\approx 20$.

### S4.3. Results for small values of n

Figure S3 displays the TDR of $\widehat{\mathrm{BH}}$ and $\mathrm{BH}^*$ for $n \in \{5, 10\}$ and $\mu \in \{1, 3, 4\}$ in the fully dense case where $m_1 = m$. In this case, when $\mu$ is large, there are $k = m$ detectable alternatives, so that the rule of thumb $n = m/(\alpha k)$ reads $n = 1/\alpha = 5$ here. We indeed observe that $\widehat{\mathrm{BH}}$ as a power close to the one of the oracle for $n = 5$ (even more for $n = 10$) when $\mu \in \{3, 4\}$, regardless of $m$. This once again suggests that the rule of thumb is valid without tuning any constant.

### S4.4. Results for bbBH procedure

This section describes the numerical experiment discussed in Section A.

First, we describe in detail the third procedure (locfdr): it is based on $\ell$-values $\ell_i = \pi_0 g_0(T_i)/g(T_i)$, $1 \leq i \leq m$, where $\pi_0$ is the probability that a null hypothesis is true and using the notation of Section A. Note that the latter is not well defined in our setting since the null hypothesis are not random. Indeed, $\ell$-values are generally defined in the so-called "two group model" (Efron et al., 2001) that uses an additional mixture effect for the configuration vector $\theta = (\theta_i)_{1 \leq i \leq m} \in \{0, 1\}^m$ with $\theta_i = 0$ if and only if $i$-th null hypothesis is true. Nevertheless, we can fix $\pi_0$ to the value $m_0/m$ and compute the $\ell$-values accordingly. Then, the version of the local FDR procedure controlling the FDR (introduced in Sun and Cai (2007)) reads as follows:

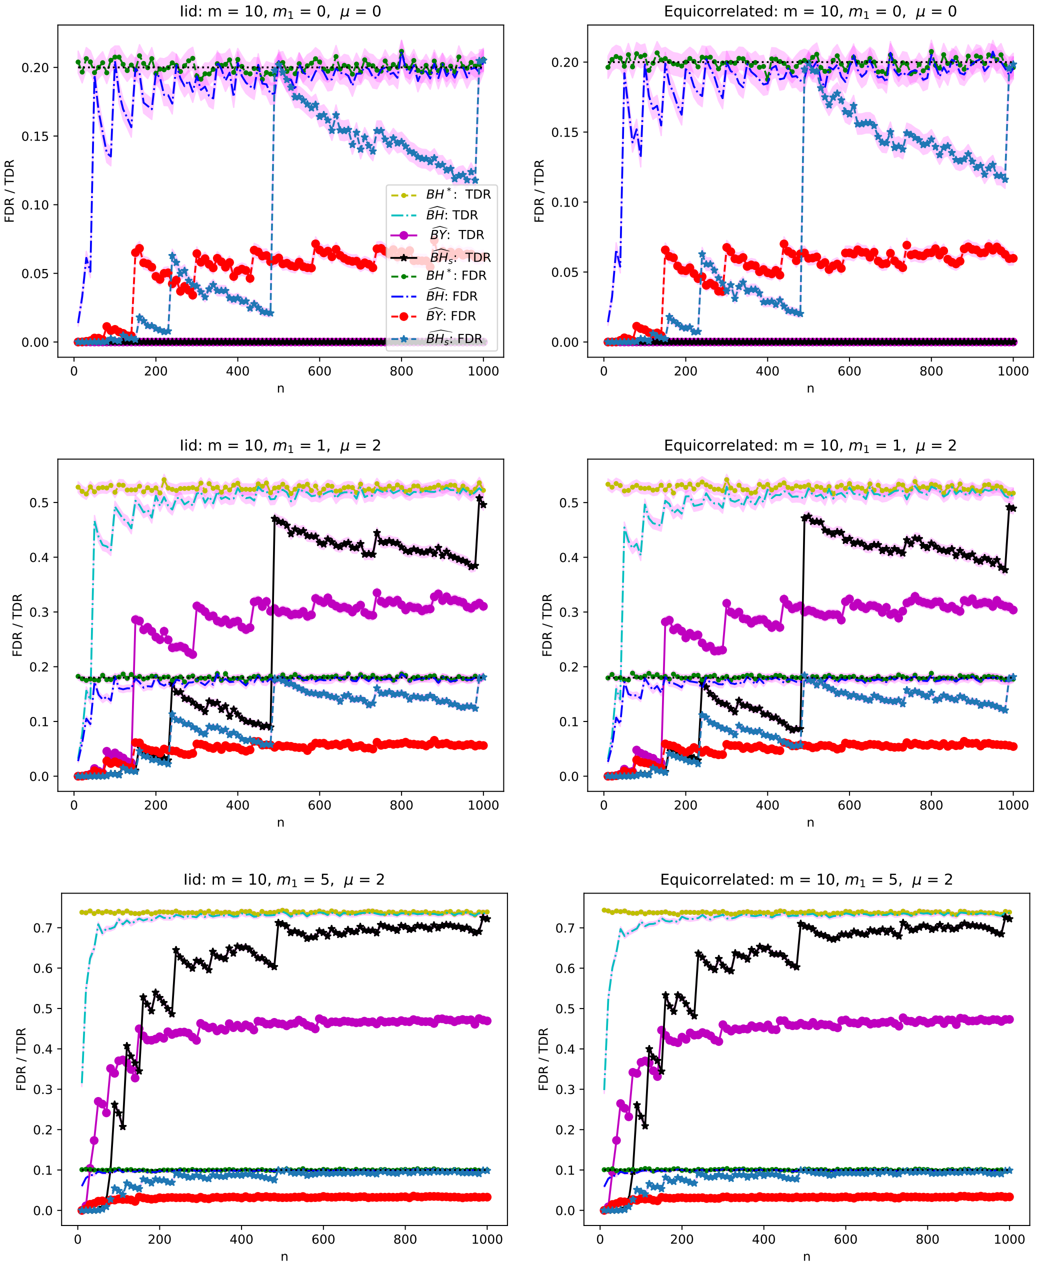


FIG S1. *Comparison with naive procedures for $m = 10$ as a function of n, for $\alpha = 0.2$. The plots display the FDR and TDR results for $BH^*$ (dark green and khaki), $\widehat{BH}$ (dark blue and cyan), $\widehat{BY}$ (red and magenta) and $\widehat{BH}_{Split}$ (gray-blue and black). Left column: i.i.d. samples. Right column: equicorrelated Gaussian samples (see Section 6.2). Top row: full null configuration, middle row: sparse case ($m_1 = 1$), bottom row: dense case ($m_1 = 5$). The number of Monte Carlo simulations used for estimating the FDR and TDR is $10^4$ for all plots. The $2\sigma$ confidence interval on the estimated FDR and TDR, when visible, is plotted in magenta.*

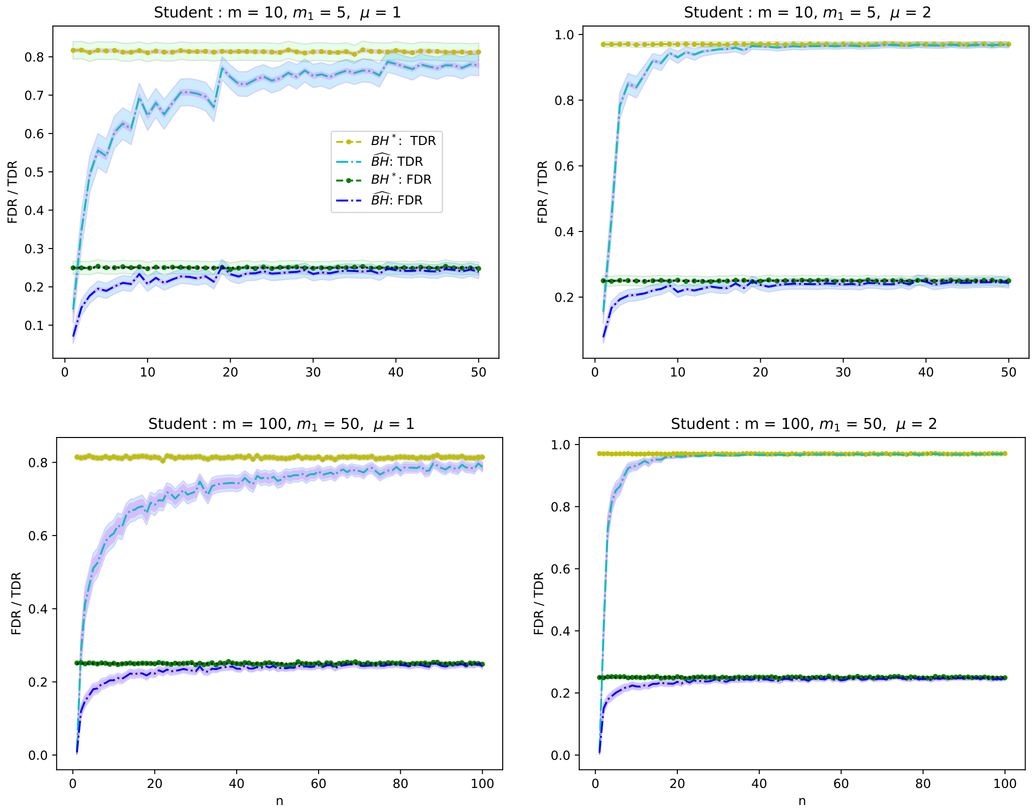


Fig S2. *FDR and TDR results for a Student distribution with three degrees of freedom, in the dense case (compare to Figure 5)* : $m_1 = \frac{m}{2}$, *with* $\mu = 1$ *(left column) and* $\mu = 2$ *(right column). The number of tests* $m$ *equals* 10 *in the top row and* 100 *in the bottom row. The number of Monte Carlo simulations used for estimating the FDR and TDR is* $10^4$ *(top row) and* $10^3$ *(bottom row). The* $2\sigma$ *confidence interval on the estimated FDR and TDR is plotted in magenta. In all plots the standard deviation (divided by* 10*) of the FDP and TDP are shown in shaded green for* $BH^*$ *and shaded blue for* $\widehat{BH}$.

- first order the $\ell$-values $\ell_{(1)} \leq \cdots \leq \ell_{(m)}$;
- reject the null corresponding to the $\hat{k}$ smallest $\ell$-values where

$$\hat{k} = \max\left\{k \in \{0, \ldots, m\} \; : \; k^{-1} \sum_{i=1}^{k} \ell_{(i)} \leq \alpha\right\}.$$

Since the value of $m_0/m$ is used in this locfdr procedure and to make the comparison fair with BH0, bbBH and BH$^*$, we apply the locfdr at level $\alpha/(m_0/m)$. This way, all procedures uses the same parameter informations and target the same FDR level $\alpha m_0/m$.

Figure S4 displays the FDP/TDP achieved by each procedure, in a Gaussian setting where $g_0$ is the density of the $\mathcal{N}(0,1)$ and $g_1$ is the density of the Cauchy distribution with mean $\mu$, taken in the range $\{1, 2, 3, 4\}$.

## References

Efron, B., R. Tibshirani, J. D. Storey, and V. Tusher (2001). Empirical Bayes analysis of a microarray experiment. *J. Amer. Statist. Assoc. 96*(456), 1151–1160.

Sun, W. and T. T. Cai (2007). Oracle and adaptive compound decision rules for false discovery rate control. *J. Am. Stat. Assoc. 102*(479), 901–912.

Tsybakov, A. B. (2009). *Introduction to nonparametric estimation.* Springer Series in Statistics. Springer, New York. Revised and extended from the 2004 French original, Translated by Vladimir Zaiats.

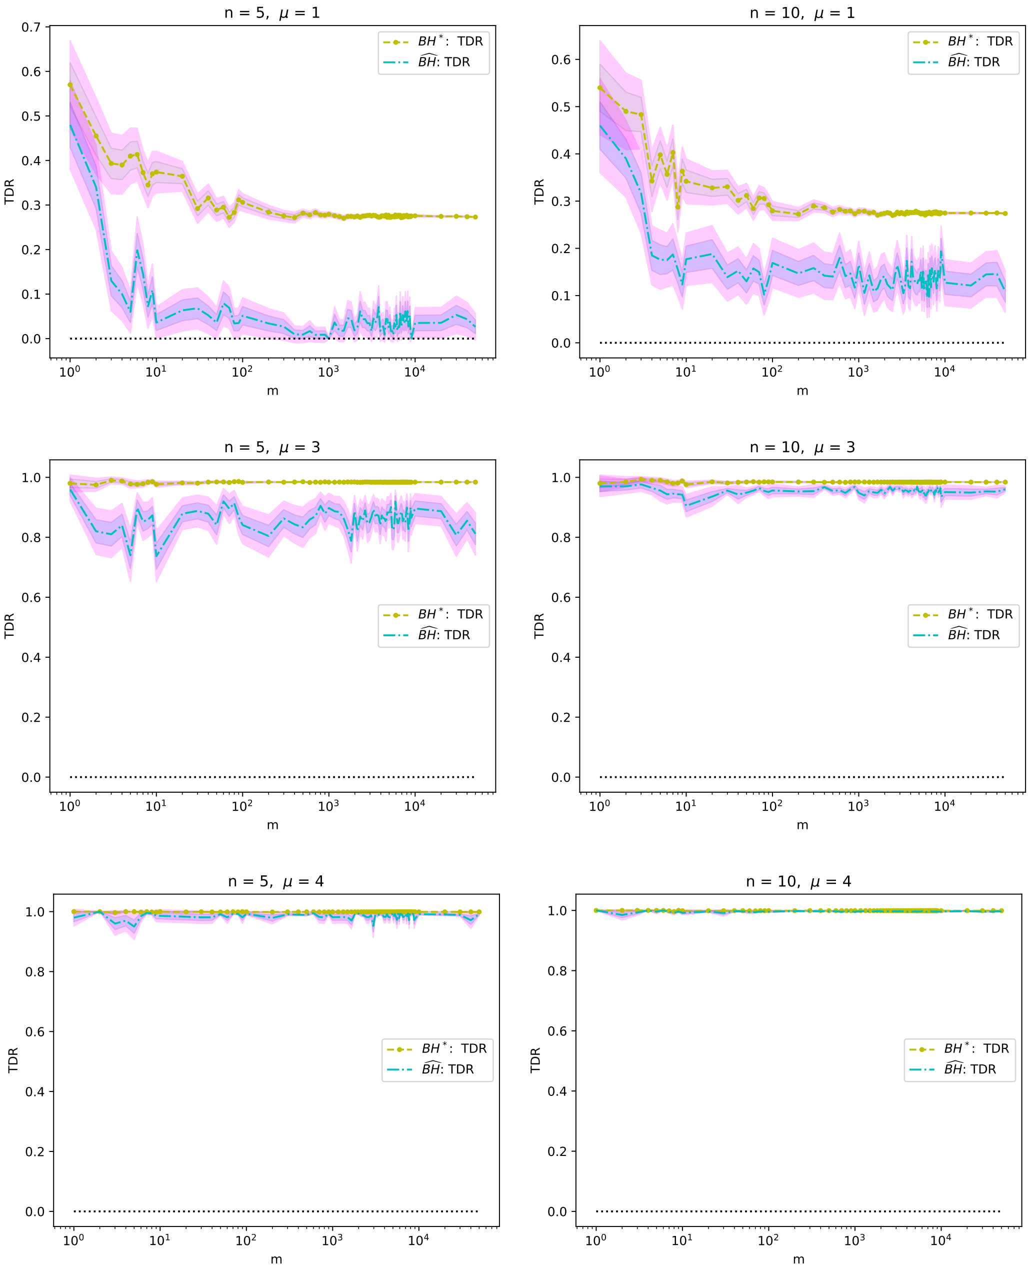


FIG S3. *TDR of* $\widehat{BH}$ $(\alpha = 0.2)$ *in the fully dense case* $m_1 = m$ *at fixed* $n = 5$ *(left column) and* $n = 10$ *(right column) for* $m$ *varying in the range* $[1\ 5 \times 10^4]$. *The signal amplitude* $\mu$ *increases from* $\mu = 1$ *(top row) to* $\mu = 3$ *(bottom row). The plots display the TDR results for* $BH^*$ *(khaki) and* $\widehat{BH}$ *(cyan). The number of Monte Carlo simulations used for estimating TDR is* $10^2$ *for all plots. The standard deviation (divided by 10) of the FDP is shown in shaded blue and the* $2\sigma$ *confidence interval on the estimated TDR is plotted in magenta.*

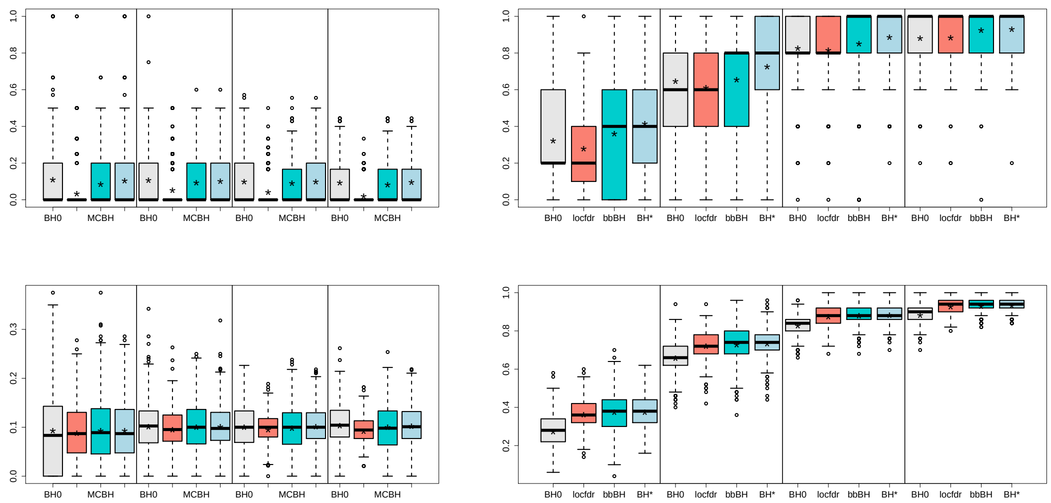


Fig S4. *Boxplots of the FDP (left) and TDP (right) for the procedures BH*0*, bbBH, Locfdr, BH*$^*$*, see text. For each boxplot, the FDR (left) and TDR (right) are depicted with the symbol "*$\star$*". Each picture is composed of* 4 *panels, one for each value of the alternative mean* $\mu \in \{1, 2, 3, 4\}$*. Top* $m = 10$*, Bottom* $m = 100$*.* $\alpha = 0.2$*,* $m_0 = m/2$*,* 500 *replications.*
